# Supplementary material for: Dynamics and Thermodynamics of a Novel Phase of NaAlH4
Source: arXiv:0910.2760 source file (2009-10-15)
Supplement: Supplementary file 1 [file supplementary.pdf]

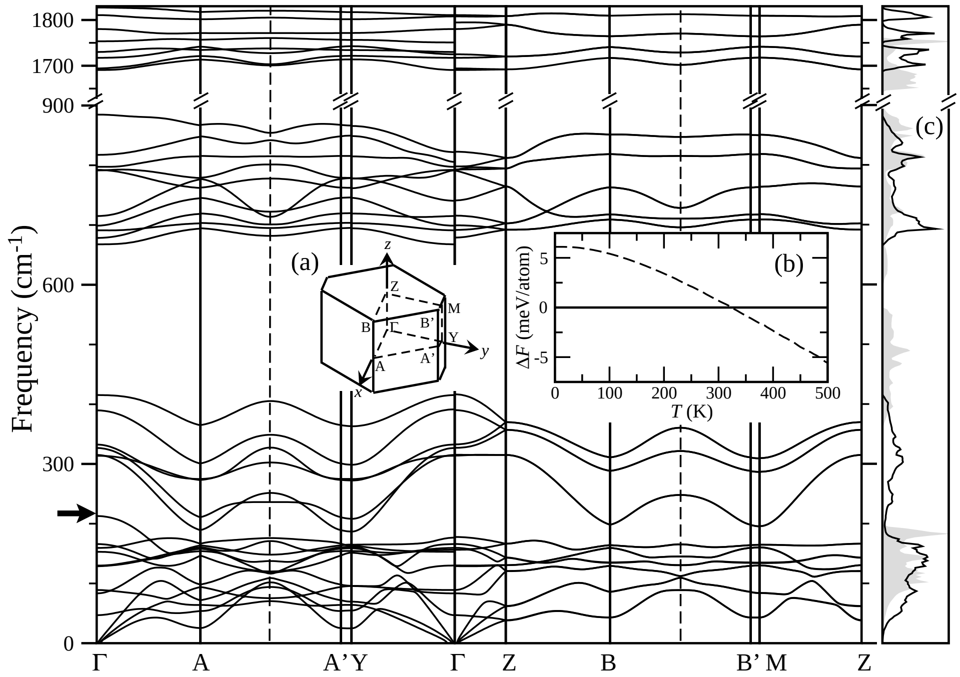


FIG. 1: Phonon dispersion of $\gamma$-$NaAlH_4$ calculated along the high-symmetry directions depicted in (a). The solid arrow indicates the highest frequency of occupied bands at the $\alpha \to \gamma$ transition temperature. Inset (b) shows the temperature-dependent free-energy difference $\Delta F = F_\gamma - F_\alpha$ between the two phases. Panel (c) compares the phonon densities of states for the $\gamma$ (solid line) and

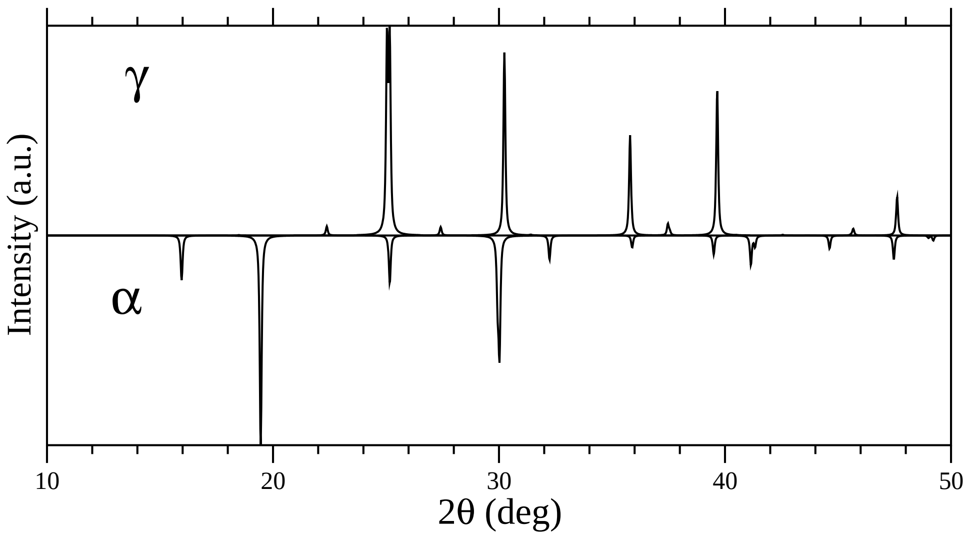


FIG. 2: Simulated X-ray diffraction data for $\gamma$-$NaAlH_4$ (top) and $\alpha$-$NaAlH_4$ (bottom).

TABLE I: Locations and relative intensities of the Raman peaks for the $\alpha$ phase of $NaAlH_4$.

| Shift (cm $^{-1}$) | Intensity (a.u.) |
|---|---|
| 118 | 7.5 |
| 120 | 9.5 |
| 187 | 15.4 |
| 189 | 43.3 |
| 459 | 90.5 |
| 561 | 59.0 |
| 745 | 46.3 |
| 792 | 94.9 |
| 813 | 4.4 |
| 845 | 54.8 |
| 1677 | 1055.8 |
| 1702 | 223.1 |
| 1747 | 4874.4 |

TABLE II: Locations and relative intensities of the Raman peaks for the $\gamma$ phase of $NaAlH_4$.

| Shift (cm $^{-1}$) | Intensity (a.u.) |
|---|---|
| 47 | 0.2 |
| 83 | 1.6 |
| 89 | 1.9 |
| 130 | 0.2 |
| 159 | 1.7 |
| 166 | 2.3 |
| 314 | 3.3 |
| 315 | 0.3 |
| 332 | 19.4 |
| 691 | 52.4 |
| 715 | 4.6 |
| 791 | 5.7 |
| 792 | 102.7 |
| 797 | 57.6 |
| 1691 | 947.5 |
| 1717 | 1573.0 |
| 1780 | 437.3 |
| 1811 | 3147.3 |
